# Supplementary material for: PyramidDrop: Accelerating Your Large Vision-Language Models via Pyramid Visual Redundancy Reduction
Source: arXiv:2410.17247 source file (2025-02-27)
Supplement: Supplementary file 1 [file appendix.tex]

% CVPR 2025 Paper Template; see https://github.com/cvpr-org/author-kit

\documentclass[10pt,twocolumn,letterpaper]{article}

%%%%%%%%% PAPER TYPE  - PLEASE UPDATE FOR FINAL VERSION
% \usepackage{cvpr}              % To produce the CAMERA-READY version
\usepackage[review]{cvpr}      % To produce the REVIEW version
\usepackage{url}
\usepackage{graphicx} 
\usepackage{booktabs}
\usepackage{makecell}

\usepackage{array}
\usepackage{multirow}
\usepackage{colortbl}

\usepackage[dvipsnames]{xcolor}

 % highlight color
 % highlight color

% Added
\usepackage[ruled]{algorithm2e}
\usepackage{bbm}
\usepackage{bm}
\usepackage{color}

\usepackage{diagbox}
\usepackage{bbding}

\usepackage{tabularx}
\usepackage{dashrule}
\usepackage[accsupp]{axessibility} % Improves PDF readability for those with disabilities.

% Import additional packages in the preamble file, before hyperref
\input{preamble}

% It is strongly recommended to use hyperref, especially for the review version.
% hyperref with option pagebackref eases the reviewers' job.
% Please disable hyperref *only* if you encounter grave issues, 
% e.g. with the file validation for the camera-ready version.
%
% If you comment hyperref and then uncomment it, you should delete *.aux before re-running LaTeX.
% (Or just hit 'q' on the first LaTeX run, let it finish, and you should be clear).
\definecolor{cvprblue}{rgb}{0.21,0.49,0.74}
\usepackage[pagebackref,breaklinks,colorlinks,allcolors=cvprblue]{hyperref}

%%%%%%%%% PAPER ID  - PLEASE UPDATE
 % *** Enter the Paper ID here

%%%%%%%%% TITLE - PLEASE UPDATE
\title{Conical Visual Concentration for Efficient Large Vision-Language Models}

%%%%%%%%% AUTHORS - PLEASE UPDATE
\author{First Author\\
Institution1\\
Institution1 address\\
{\tt\small firstauthor@i1.org}
% For a paper whose authors are all at the same institution,
% omit the following lines up until the closing ``}''.
% Additional authors and addresses can be added with ``\and'',
% just like the second author.
% To save space, use either the email address or home page, not both
\and
Second Author\\
Institution2\\
First line of institution2 address\\
{\tt\small secondauthor@i2.org}
}

% \begin{document}
% % \maketitle

% \end{document}

\begin{document}
\input{sec/X_suppl}
{
    \small
    \bibliographystyle{ieeenat_fullname}
    \bibliography{main}
}
\end{document}
